# Supplementary material for: Building Intelligent Autonomous Navigation Agents
Source: arXiv:2106.13415 source file (2021-06-25)
Supplement: Supplementary file 1 [file appendix.tex]

\section{Background: Reinforcement Learning}
\label{sec:rl}
In the standard Reinforcement Learning \cite{sutton1998reinforcement} setting, at each time step $t$, an agent receives a observation, $s_t$, from the environment, performs an action $a_t$ and receives a reward $r_t$. The goal is to learn a policy $\pi(a|s)$ which maximizes the expected return or the sum of discounted rewards $R_t = \Sigma_{t'=t}^T \gamma^{t'-t} r_{t'}$,
where T is the time at which the episode terminates, and $\gamma \in \left[ 0, 1\right]$ is a discount factor that determines the importance of future rewards.

Reinforcement learning methods can broadly be divided into value-based methods and policy-based methods. Policy-based methods parametrize the policy function which can be optimized directly to maximize the expected return ($\mathbb{E}[R_t]$) \cite{sutton2000policy}. While policy-based methods suffer from high variance, value-based methods typically use temporal difference learning which provides low variance estimates of the expected return. Actor-Critic methods \citep{barto1983neuronlike, sutton1984temporal, konda1999actor} combine the benefits of both value-based methods by estimating both the value function, $V^\pi(s_t;\theta_v)$, as well as the policy function $\pi(a_t|s_t;\theta)$\citep{grondman2012survey}. 

REINFORCE family of algorithms \citep{williams1992simple} are popular for optimizing the policy function, which updates the policy parameters $\theta$ in the direction of $\nabla_{\theta} \log \pi(a_t|s_t;\theta)R_t$. Since this update is an unbiased estimate of  $\nabla_\theta\mathbb{E}[R_t]$, its variance can be reduced by subtracting a baseline function, $b_t(s_t)$ from the expected return ($\nabla_{\theta} \log \pi(a_t|s_t;\theta)(R_t-b_t(s_t))$). When the estimate of the value function ($V^\pi(s_t)$) is used as the baseline, the resultant algorithm is called Advantage Actor-Critic, as the resultant policy gradient is scaled by the estimate of the \textit{advantage} of the action $a_t$ in state $s_t$, $A(a_t,s_t) = Q(a_t,s_t) - V(s_t)$. The Asynchronous Advantage Actor-Critic algorithm \citep{mnih2016asynchronous} uses a deep neural network to parametrize the policy and value functions and runs multiple parallel threads to update the network parameters.

In this paper, we use the A3C algorithm for all our experiments. We also use entropy regularization for improved exploration as described by \citep{mnih2016asynchronous}. In addition, we use the Generalized Advantage Estimator \citep{schulman2015high} to reduce the variance of the policy gradient updates.

\section{Implementation Details}
\label{sec:implementation}
\subsection{Model Architecture Details}
The \textbf{perceptual model} for the 3D Environments receives RGB images of size 108x60. It consists of 2 Convolutional Layers. The first convolutional layer contains 32 filters of size 8x8 and stride of 4. The second convolutional layer contains 64 filters of size 4x4 with a stride of 2. The convolutional layers are followed by a fully-connected layer of size 512. The output of this fully-connected layer is used as the representation of the image while constructing the likelihood map. Figure~\ref{fig:perceptual_arch} shows the architecture of the perceptual model in 3D environments. This architecture is adapted from previous work which is shown to perform well at playing deathmatches in Doom \citep{chaplot2017arnold}. 

The \textbf{policy model} consists of two convolutional layers too. For the 2D environments, both the convolutional layers contain 16 filters of size 3 with stride of 1. For the 3D environments, the first convolutional layer contains 16 filters of size 7x7 with a stride of 3 and the second convolutional layer contains 16 filters of size 3x3 with a stride of 1. The convolutional layers are followed by a fully-connected layer of size 256. Figure~\ref{fig:policy_arch} shows the architecture of the policy model in 3D environments. 

We add action histroy of length 5 (last 5 actions) as well as the current time step as input to the policy model. We observed that action history input avoids the agent being stuck in alternating `turn left' and `turn right' actions whereas time step helps in accurately predicting the value function as the episode lengths are fixed in each environment. Each action in the action history as well as the current timestep are passed through an Embedding Layer to get an embedding of size 8. The embeddings of all actions and the time step are contacted with the 256-dimensional output of the fully-connected layer. The resultant vector is passed through two branches of single fully-connected layers to get the policy (actor layer with 3 outputs) and the value function (critic layer with 1 output). 

\begin{figure*}
\centering
\includegraphics[width=0.80\linewidth,height=\textheight,keepaspectratio]{anl/images/perceptual_arch}
%\vspace{-0.5em}
\caption{\small Figure showing the architecture of the perceptual model in 3D Environments.}
\label{fig:perceptual_arch}
\end{figure*}

\begin{figure*}
\centering
\includegraphics[width=0.99\linewidth,height=\textheight,keepaspectratio]{anl/images/policy_arch}
%\vspace{-0.5em}
\caption{\small Figure showing the architecture of the policy model in 3D Environments.}
\label{fig:policy_arch}
\end{figure*}

\subsection{Hyper-parameters and Training Details}
All the models are trained with A3C using Stochastic Gradient Descent with a learning rate of 0.001. We use 8 threads for 2D experiments and 4 threads for 3D experiments. Each thread performed an A3C update after 20 steps.  The weight for entropy regularization was 0.01. The discount factor ($\gamma$) for reinforcement learning was chosen to be 0.99. The gradients were clipped at 40. All models are trained for 24hrs of wall clock time. All the 2D experiments (including evaluation runtime benchmarks for baselines) were run on Intel(R) Xeon(R) CPU E5-2630 v4 @ 2.20GHz and all the 3D experiments were run on Intel(R) Core(TM) i7-6850K CPU @ 3.60GHz. While all the A3C training threads ran on CPUs, the Unreal engine also utilized a NVidia GeForce GTX 1080 GPU. The model with the best performance on the training environment is used for evaluation.

\subsection{Transition function}
The transition function transforms the belief according to the action taken by the agent. For turn actions, the beliefs maps in each orientation are swapped according to the direction of the turn. For the move forward action, all probability values move one cell in the orientation of the agent, except those which are blocked by a wall (indicating a collision). Figure~\ref{fig:motion_model} shows sample outputs of the transition function given previous belief and action taken by the agent. 
\begin{figure*}[h]
\centering
%% \vspace{-0.5em}
\includegraphics[width=0.99\linewidth,height=\textheight,keepaspectratio]{anl/images/motion_model}
\caption{Sample output of the transition function ($f_T$) given previous belief and action taken by the agent. The map design is shown in the left.}
\label{fig:motion_model}
\end{figure*}

\subsection{Implementation details of Active Markov Localization}
In order to make our implementation of generalized AML as efficient as possible, we employ various techniques described by the authors, such as Pre-computation and Selective computation \citep{fox1998active}, along with other techniques such as hashing of expected entropies for action subsequences. The restrictions in runtime led to $n_l=1,n_g=1,n_m=5$ in both 2D and 3D environments for AML (Fast), $n_l=5,n_g=1,n_m=10$ in 2D environments for AML (Slow) and $n_l=3,n_g=3,n_m=10$ in the 3D environments for AML (Slow).

The computation of expected entropies require the expected observation in the future states while rolling out a sequence of action. While it is possible to calculate these in 2D environments with depth-based observations, it is not possible to do this in 3D environments with RGB image observations. However, for comparison purposes we assume that AML has a perfect model of the environment and provide future observations by rolling out the action sequences in the simulation environment.
